# Supplementary material for: Resilient Constrained Learning
Source: arXiv:2306.02426 source file (2024-01-11)
Supplement: Supplementary file 1 [file 08_1_1_appendix_pointwise.tex]

\section{Pointwise Constraints}~\label{a:pointwise}
Our approach together with all of the results in the main body can be extended to problems of the form
\begin{prob}[P-CSL]\label{eqn_csl_dense}
	\P ~=~  
	   &  \min_{\phi}
	      && \mbE_{(\bbx, y) \sim \calD_0} 
                \Big[ \ell_0(\phi(\bbx),y)\Big], \\
	   &  \text{~s.t.}
	      && \mbE_{(\bbx, y) \sim \calD_i} 
                \Big[ \ell_i(\phi(\bbx),y)\Big] \leq 0, \quad 
                   && i = 1, \dots, m, \\
	   &  && \ell_i(\phi(\bbx), y) \leq 0,  \quad \ccalD_i-\text{a.e.}, \quad 
                   && i = m + 1, \dots, m + q . \phantom{\Big[}
\end{prob}
The first $m$ constraints $\mbE_{(\bbx, y) \sim \calD_i} [ \ell_i(\phi(\bbx),y)] \leq 0$, with $i = 1, \dots, m$, are constraints on statistical functionals as described in the main body. The remaining $q$ constraints, with $i = m+1, \dots, m+q$, are pointwise as we require $\ell_i(\phi(\bbx), y) \leq 0$  for almost all pairs $(\bbx,y)$ drawn according to the probability distribution $\ccalD_i$. We remark that the probability distributions $\ccalD_i$ can be dense, implying that the number of constraints in \eqref{eqn_csl} can be infinite. Unlike the constraints on expected values, we require the losses $\ell_i$ to be convex. That is, in this case we require Assumption~\ref{ass_non_convex}(a) to hold. Explicitly, in what follows we replace Assumption~\ref{ass_non_convex} by the following Assumption.
\begin{assumption}[Convex Cost Constraint Set]\label{ass_non_convex_dense} 
Either
\begin{enumerate}[(a)]
    \item The loss functions $\ell_i$ $i = 0,\ldots,m+q$ are convex.
    \item \textbf{q=0}, the loss functions $\ell_i$ $i = 0,\ldots,m$ are non-convex, and either
    \begin{enumerate}[(i)]
        \item (Classification) $\mathcal{Y}$ is finite, and the conditional random variables $\bbx \mid y$ induced by the $\mathfrak{D}_i$ is non-atomic, and $\ccalF$ is decomposable.
        \item (Regression. Informally, see~\cite{non-convex}.) $\mathcal{Y}$ is compact and the losses are uniformly continuous in $y$.
    \end{enumerate}
\end{enumerate}
\end{assumption}
In this setting, we defined the relaxed problem as
\begin{prob}[P-RLX]\label{eqn_the_problem_dense}
	\P(\bbu) ~=~  
	   &  \min_{\phi}
	      && \mbE_{(\bbx, y) \sim \calD_0} 
                \Big[ \ell_0(\phi(\bbx),y)\Big], \\
	   &  \text{~s.t.}
	      && \mbE_{(\bbx, y) \sim \calD_i} 
                \Big[ \ell_i(\phi(\bbx),y)\Big] \leq u_i, \quad 
                   && i = 1, \dots, m, \\
	   &  && \ell_i(\phi(\bbx), y) \leq u_i(\bbx),  \quad \ccalD_i-\text{a.e.}, \quad 
                   && i = m + 1, \dots, m + q , \phantom{\Big[}
\end{prob}
where now the perturbations $u_i(\bbx)$, for $i = m + 1, \dots, m + q$ are $\ccalD_i$-square-measurable function taking non-negative values $u_i(\bbx) \geq 0$.
The perturbation function $P(\bbu)$ is convex, as shown in~\ref{prop:pert_cvx}. Analogous to the subdifferential in Definition~\ref{def_subdifferential}, this latter fact permits definition of a global Fr\'echet subdifferential,  as we formulate next. 
\begin{definition}\label{def_subdifferential_dense} 
Given the convex perturbation function $\P(\bbu)$, its Fr\'echet subdifferential $\Fre \P(\bbu)$ is the set of all Fr\'echet subgradients $\bbw$ such that for all $\bbv$ it holds
\begin{align}\label{eqn_subdifferential_dense}
   \P(\bbv) 
      \geq \P(\bbu) 
              + \Big\langle \bbw, \bbv - \bbu \Big\rangle, 
\end{align} 
where $\langle \bbw, \bbv - \bbu \rangle = \sum_{i=1}^{m} \bbw_i (v_i-u_i) + \sum_{i=m+1}^{m+q}  \mbE_{\ccalD_i} [\bbw_i(\bbx) (\bbv_i(\bbx)-\bbu_i(\bbx)]$ denotes the inner product of $\bbw$ and $\bbv-\bbu$. 
\end{definition}
Then all of our previous results can be extended to pointwise constraints by replacing subdifferentials by Fr\'echet (directional) subdiferentials. Namely, we let $h(\bbu)$ be a Fr\'echet differentiable convex nondecreasing function and seek for the resilient relaxation defined as in~\ref{eqn_resilient_equilibrium},
\begin{prob}[P-RSL]\label{eqn_resilient_equilibrium_dense}
   -\Fre h(\bbu^{\star}) \in \Fre \P(\bbu^{\star}),
\end{prob} 
where $\Fre h(\bbu^{\star})$ now represents Fr\'echet derivative of $h$ and $\Fre \P(\bbu^{\star})$ the Fr\'echet subdifferential of the perturbation function.
%5
In the same way, optimal Lagrange multipliers are Fr\'echet subgradients of the perturbation function. To state this formally let $\bblam$ represent $m$ Lagrange multipliers $\lam_i$ for $1\leq i\leq m$ and $q$ Lagrange multiplier functions $\lam_i(\bbx)$ for $m+1\leq i\leq m+q$. We define the Lagrangian associated with \eqref{eqn_the_problem_dense} as
\begin{align}\label{eqn_Lagrangian_dense}
   \calL(\phi, \bblam; \bbu) &
      ~=~ \mbE_{\ccalD_0} \Big[ \ell_0(\phi(\bbx),y) \Big]   \\ \nonumber & \qquad
             + \sum_{i = 1}^m 
                  \lam_i \bigg [
                     \mbE_{\ccalD_i} 
                        \Big[ \ell_i(\phi(\bbx),y)\Big] - u_i  \bigg]
             + \sum_{i=m+1}^{m+q} 
                  \mbE_{\ccalD_i}
                     \bigg[ \lam_i(\bbx) \Big[\ell(\phi(\bbx),y) - u_i(\bbx) \Big] \bigg]
\end{align}
Note that in the $q$ pointwise constraints the perturbations $u_i(\bbx)$ and the Lagrange multipliers $\lam_i(\bbx)$ are inside the expectation operator. This is because the constraints are pointwise, i.e., they are required to hold for almost all $\bbx$ with respect to the distribution $\ccalD_i$.

Analogously to the finite constraint case, from the Lagrangian in \eqref{eqn_Lagrangian_dense} we construct the dual function by minimizing over the primal variable $\phi$,
\begin{equation}\label{eqn_the_dual_dense}
   g(\bblam;\bbu) = \min_{\phi} \calL(\phi, \bblam; \bbu).
\end{equation}
And we further define the dual optimum by minimizing the dual function over nonnegative multipliers,
\begin{prob}[D-RLX]\label{dual_prob_dense}
    \D(\bbu) ~=~  \max_{\bblam \succeq \bbzero } g(\bblam;\bbu)
             ~=~ g(\bblam^*(\bbu);\bbu),
\end{prob}

As shown in~\ref{pf:subdifferential}, optimal dual variables are Fr\'echet subgradients of the perturbation function of \eqref{eqn_the_problem}, i.e., proposition~\ref{prop_subdifferential} holds despite the presence of a dense set of constraints.

The remaining results in the main text also hold for pointwise constraints, considering the primal and dual problems defined above. Therefore, all of the proofs in Section~\ref{a:proofs} are presented with pointwise constraints, although they can be particularized to the results in the main body by setting $q = 0$.
